# Supplementary material for: Modelling hollow thermoplastic syntactic foams under high-strain compressive loading
Source: arXiv:1811.07193 source file (2021-03-09)
Supplement: Supplementary file 1 [file supp_mater.pdf]

# Supplementary Material for “Modelling hollow thermoplastic syntactic foams under high-strain compressive loading”

M. J. A. Smith<sup>a</sup>, Z. Yousaf<sup>a,b</sup>, P. Potluri<sup>b</sup>, W. J. Parnell<sup>a</sup>

<sup>a</sup>*School of Mathematics, University of Manchester, Oxford Rd, Manchester M13 9PL, UK*

<sup>b</sup>*Robotics and Textile Composite Group, Northwest Composite Centre, School of Materials, University of Manchester, Manchester M13 9PL, UK*

---

## SM1. Toe correction for axial stress-strain data

Toe compensation of stress-strain data was made in accordance with Appendix A1 of ASTM D695.

## SM2. Toe correction for transverse stretch data

Toe compensation was also carried out on the transverse strain data, by taking a linear least-squares fit of the logarithm of the raw axial strain data against the logarithm of the raw transverse strain data. From the resulting log-log plot, the toe region was evident at small strains before the intrinsic linear region of the material emerges. After removing data from the toe region, a straight line fit of the remaining data was made in the small-strain limit (on a log-log scale), giving the intrinsic Poisson ratio of the material (see below). Using the small-strain Poisson ratio and a model for the relationship between stretches (i.e., see the Hencky ratio definition in the main text) the toe compensation offset was determined at a specified strain threshold, by imposing continuity of small-strain approximations with the test data.

For completeness, we remark that the data was extracted as follows: video files were converted into sequences of image files and post-processed in MATLAB. Sample edges were tracked using either the contrast in pixel value or the gradient of the pixel value, depending on the brightness contrast between the material and either the platens or the background (see Fig. 2 of the main text).

|          | $C_{10}$   | $D_1$           |
|----------|------------|-----------------|
| unfilled | 1234544.97 | 1.630902779e-08 |
| 2% HTM   | 1156759.51 | 3.504664551e-08 |
| 10% HTM  | 1048263.38 | 7.840756667e-08 |
| 40% HTM  | 644550.08  | 5.557503890e-07 |

Table SM1: Non-linear least squares fit results for all HTM syntactic foams using Compressible neo-Hookean strain energy model .

| $N$        | 1              | 2              | 3             | 4              |
|------------|----------------|----------------|---------------|----------------|
| $\mu_1$    | 2332289.98     | 3157986.42     | 3624720.8     | 3547300.05     |
| $\mu_2$    | -              | -851231.413    | -1725876.81   | -1665262.4     |
| $\mu_3$    | -              | -              | 395252.993    | 424302.781     |
| $\mu_4$    | -              | -              | -             | -11275.0462    |
| $\alpha_1$ | 0.67916733     | -0.21213547    | 2.00024015    | 2.00033378     |
| $\alpha_2$ | -              | -1.47293207    | 4.00020814    | 4.00019132     |
| $\alpha_3$ | -              | -              | -1.99990877   | -2.00013001    |
| $\alpha_4$ | -              | -              | -             | -4.00001302    |
| $D_1$      | 1.72656302e-08 | 1.74567547e-08 | 1.7553075e-08 | 1.75456684e-08 |
| $D_2$      | -              | 0              | 0             | 0              |
| $D_3$      | -              | -              | 0             | 0              |
| $D_4$      | -              | -              | -             | 0              |

Table SM2: Non-linear least squares fit results for unfilled foam using Ogden Type-I strain energy model

| $N$        | 1              | 2             | 3              | 4              |
|------------|----------------|---------------|----------------|----------------|
| $\mu_1$    | 2314436.13     | 2346298.3     | 2374673.78     | 185169.493     |
| $\mu_2$    | -              | -10.207       | -10556.8346    | 1713808.79     |
| $\mu_3$    | -              | -             | -36595.2646    | 773011.909     |
| $\mu_4$    | -              | -             | -              | -315304.131    |
| $\alpha_1$ | 2.01390018     | 2.42208855    | 1.99813073     | 2.00001638     |
| $\alpha_2$ | -              | -17.59339200  | 4.00000380     | 3.99980057     |
| $\alpha_3$ | -              | -             | -2.00062201    | -2.00017643    |
| $\alpha_4$ | -              | -             | -              | -4.00024482    |
| $D_1$      | 3.50327581e-08 | 3.4557172e-08 | 3.48358006e-08 | 3.44047018e-08 |
| $D_2$      | -              | 0             | 0              | 0              |
| $D_3$      | -              | -             | 0              | 0              |
| $D_4$      | -              | -             | -              | 0              |

Table SM3: Non-linear least squares fit results for 2% HTM syntactic foam using Ogden Type-I strain energy model

| $N$        | 1             | 2              | 3              | 4              |
|------------|---------------|----------------|----------------|----------------|
| $\mu_1$    | 2114914.86    | 2961177.71     | 2065793.82     | -9599605.94    |
| $\mu_2$    | -             | -424464.592    | 2171817.06     | 7107023.38     |
| $\mu_3$    | -             | -              | -1673875.92    | 11646131.5     |
| $\mu_4$    | -             | -              | -              | -6591593.51    |
| $\alpha_1$ | 2.34110133    | 5.64226440     | -1.62252958    | 2.52618471     |
| $\alpha_2$ | -             | -4.39449282    | 8.60155676     | 5.48335761     |
| $\alpha_3$ | -             | -              | -3.95721380    | -0.65704653    |
| $\alpha_4$ | -             | -              | -              | -2.18537226    |
| $D_1$      | 7.7725853e-08 | 6.48017943e-08 | 6.41187812e-08 | 6.41633194e-08 |
| $D_2$      | -             | 0              | 0              | 0              |
| $D_3$      | -             | -              | 0              | 0              |
| $D_4$      | -             | -              | -              | 0              |

Table SM4: Non-linear least squares fit results for 10% HTM syntactic foam using Ogden Type-I strain energy model

| $N$        | 1              | 2             | 3              | 4              |
|------------|----------------|---------------|----------------|----------------|
| $\mu_1$    | 1293707.93     | 6310300.11    | 1115950.12     | -35753384      |
| $\mu_2$    | -              | -2753415.89   | 6043661.87     | 27423862.9     |
| $\mu_3$    | -              | -             | -3033593.34    | 20048488.3     |
| $\mu_4$    | -              | -             | -              | -7624319.05    |
| $\alpha_1$ | 2.12108960     | 11.10980850   | 0.85229272     | 5.99601048     |
| $\alpha_2$ | -              | -5.76362506   | 21.03944300    | 10.86791790    |
| $\alpha_3$ | -              | -             | -10.51367650   | 0.83295936     |
| $\alpha_4$ | -              | -             | -              | -5.95490946    |
| $D_1$      | 5.53770981e-07 | 2.0141727e-07 | 1.73634191e-07 | 1.74964459e-07 |
| $D_2$      | -              | 0             | 0              | 0              |
| $D_3$      | -              | -             | 0              | 0              |
| $D_4$      | -              | -             | -              | 0              |

Table SM5: Non-linear least squares fit results for 40% HTM syntactic foam using Ogden Type-I strain energy model

| $N$        | 1           | 2            | 3            | 4            |
|------------|-------------|--------------|--------------|--------------|
| $\mu_1$    | 2.51036e+06 | 5.48856e+06  | 4.0948e+07   | 1.24836e+09  |
| $\mu_2$    | -           | -1.34469e+06 | -3.61566e+07 | -2.78565e+09 |
| $\mu_3$    | -           | -            | -641284      | 2.5495e+09   |
| $\mu_4$    | -           | -            | -            | -1.00776e+09 |
| $\alpha_1$ | 5.90359     | 12.48340     | 7.32316      | 4.62578      |
| $\alpha_2$ | -           | -2.38927     | 6.45122      | 3.76908      |
| $\alpha_3$ | -           | -            | -3.02242     | 2.66095      |
| $\alpha_4$ | -           | -            | -            | 1.94116      |
| $\nu_1$    | 0.229254    | 0.227158     | 0.192050     | 0.285315     |
| $\nu_2$    | -           | 1.205290     | 0.174439     | 0.288010     |
| $\nu_3$    | -           | -            | 4.057170     | 0.289337     |
| $\nu_4$    | -           | -            | -            | 0.287765     |

Table SM6: Non-linear least squares fit results for 40% HTM syntactic foam using Ogden Type-II strain energy model

## 27 SM4. Small-strain constants for fitted models

28 For a Compressible neo-Hookean model, the model coefficients are related to the ground-  
 29 state constants via

$$G_0 = 2C_{10} \quad K_0 = 2/D_1, \quad (1)$$

30 whereas for a Compressible Ogden type-I model,  $\mu_j$ ,  $\alpha_j$ , and  $D_j$  are related to ground-state  
 31 constants via

$$G_0 = \sum_{k=1}^N \mu_k, \quad K_0 = 2/D_1, \quad (2)$$

32 and finally, for Compressible Ogden type-II model, the real-valued coefficients  $\alpha_k$ ,  $\beta_k$ , and  $\mu_k$   
 33 are related to ground state constants by

$$G_0 = \sum_{k=1}^N \mu_k, \quad K_0 = \sum_{k=1}^N 2\mu_k \left( \beta_k + \frac{1}{3} \right). \quad (3)$$

34 For reference, we remark that the data for Compressible Ogden type-II model is represented  
 35 by  $\nu_k$  in place of  $\beta_k$ , however, these are trivially related by  $\beta_k = \nu_k/(1 - 2\nu_k)$ .

36 For ease of comparison to experimentally obtained data, we calculate the small-strain  
 37 Poisson ratio  $\nu_0$  and the Young's modulus  $Y_0$  using the relations

$$\nu_0 = \frac{(3K_0 - 2G_0)}{2(3K_0 + G_0)}, \quad Y_0 = \frac{9K_0G_0}{3K_0 + G_0}. \quad (4)$$

38 with results tabulated overleaf.

|     |          | $Y_0$ [MPa] | $\nu_0$ |
|-----|----------|-------------|---------|
| 0%  | CnH      | 7.36        | 0.49    |
|     | OgI:1    | 6.95        | 0.49    |
|     | OgI:2    | 6.87        | 0.49    |
|     | OgI:3    | 6.84        | 0.49    |
|     | OgI:4    | 6.84        | 0.49    |
| 2%  | CnH      | 6.85        | 0.48    |
|     | OgI:1    | 6.85        | 0.48    |
|     | OgI:2    | 6.95        | 0.48    |
|     | OgI:3    | 6.89        | 0.48    |
|     | OgI:4    | 6.98        | 0.48    |
| 10% | CnH      | 6.12        | 0.46    |
|     | OgI:1    | 6.18        | 0.46    |
|     | OgI:2    | 7.3         | 0.46    |
|     | OgI:3    | 7.49        | 0.46    |
|     | OgI:4    | 7.48        | 0.46    |
| 40% | CnH      | 3.45        | 0.34    |
|     | OgI:1    | 3.47        | 0.34    |
|     | OgI:2    | 9.53        | 0.34    |
|     | OgI:3    | 11.06       | 0.34    |
|     | OgI:4    | 10.97       | 0.34    |
|     | OgII:1-4 | 11.94       | 0.343   |

Table SM7: Small-strain values for Young's modulus  $Y_0$  and Poisson's ratio  $\nu_0$  obtained using fitted model coefficients.
